# Supplementary material for: Fine-grained 3D object recognition: an approach and experiments
Source: arXiv:2306.15919 source file (2023-06-28)
Supplement: Supplementary file 1 [file appendixA.tex]

\section{Appendix}\label{ap:appendix}
In the Appendix (or Appendices) you may give the details that did not fit in the main text. If necessary, you may use a one-column lay-out here. Start the first appendix on a new page.
