# Supplementary material for: Fine-grained 3D object recognition: an approach and experiments
Source: arXiv:2306.15919 source file (2023-06-28)
Supplement: Supplementary file 2 [file appendixB.tex]

\section{Appendices}\label{ap:appendices}
If you have more than one Appendix, use letters to ‘‘number” them. You may start every appendix on a new page, but this is not necessary. If you have many appendices, it may be helpful for the reader to have a list of appendices on the first page of the appendices.
